# Supplementary material for: NeAT: Neural Adaptive Tomography
Source: arXiv:2202.02171 source file (2022-02-04)
Supplement: Supplementary file 1 [file 8_Appendix.tex]

% Appendix
\appendix
